# Supplementary material for: Chiral symmetry constraints on resonant amplitudes
Source: arXiv:1707.08983 source file (2018-01-27)
Supplement: Supplementary file 1 [file SupplementalProofs.pdf]

### A. Generalities

We consider here the residue of the quadruple pion pole in the pseudoscalar four-point function, i.e.

$$G^{abcd}(q_j) := i^3 \int d^4x_1 d^4x_2 d^4x_3 \, e^{i(q_a x_1 + q_b x_2 - q_c x_3)} \langle 0|TP^a(x_1)P^b(x_2)P^c(x_3)P^d(0)|0\rangle \,,$$

$$G^{abcd}_{\rm res}(q_j) := \left(\prod_{j=a}^{d} \lim{}_{q_j^2 \to M_\pi^2}(q_j^2 - M_\pi^2)\right) G^{abcd}(q_j)\,, \quad j = a, b, c, d, \tag{1}$$

compare Sec. 16 of [1] (see also Sec. 4.6.2 of [2]). Note that $q_d = q_a + q_b - q_c$ (energy-momentum conservation). Using isospin and crossing symmetry, this can be written as

$$\begin{aligned} G^{abcd}_{\rm res}(q_j) &= G_\pi^4 \left(A(s,t,u)\delta^{ab}\delta^{cd} + A(t,u,s)\delta^{ac}\delta^{bd} + A(u,s,t)\delta^{ad}\delta^{bc}\right) \\ &\equiv G_\pi^4 T^{abcd}(s,t)\,, \end{aligned} \tag{2}$$

where the first factor is related to the matrix element of a pion with the pseudoscalar current,

$$\langle 0|P^a(x)|\pi^b(q)\rangle = \delta^{ab} e^{-iqx} G_\pi\,, \tag{3}$$

while the second factor is the on-shell scattering amplitude for the process $\pi^a(q_a)\pi^b(q_b) \to \pi^c(q_c)\pi^d(q_d)$, with $s = (p_a + p_b)^2\,, \quad t = (p_a - p_c)^2\,, \quad u = 4M_\pi^2 - s - t\,.$

Moreover, we note that the matrix element

$$\mathcal{M}^{ef}_{abcd}(x_j) := \langle \pi^f(p')|TP^a(x_1)P^b(x_2)P^c(x_3)P^d(0)|\pi^e(p)\rangle \tag{4}$$

is related to the above four-point function in the limit where $M_\pi \to 0$ (chiral limit) and $p', p \to 0$,

$$\begin{aligned} \overline{\mathcal{M}}^{ef}_{abcd}(x_j) &:= \lim{}_{p,p'\to 0} \lim{}_{M_\pi \to 0} \mathcal{M}^{ef}_{abcd}(x_j) \qquad (5) \\ &= -\frac{1}{2F^2}\Big( \delta^{af}\langle 0|TP^e(x_1)P^b(x_2)P^c(x_3)P^d(0)|0\rangle \\ &\quad + \delta^{bf}\langle 0|TP^a(x_1)P^e(x_2)P^c(x_3)P^d(0)|0\rangle \\ &\quad + \delta^{cf}\langle 0|TP^a(x_1)P^b(x_2)P^e(x_3)P^d(0)|0\rangle \\ &\quad + \delta^{df}\langle 0|TP^a(x_1)P^b(x_2)P^c(x_3)P^e(0)|0\rangle + (e \leftrightarrow f) + \ldots \Big)\Big|_{M_\pi \to 0}\,, \end{aligned}$$

where the dots stand for terms not leading to four pion poles in the Fourier transform, and $F$ is the pion decay constant in the chiral limit. See App. A for a short derivation.

The Fourier transform of $\overline{\mathcal{M}}^{ef}_{abcd}(x_j)$ is thus of the form

$$\overline{M}^{ef}_{abcd}(q_j) := i^3 \int d^4x_1 d^4x_2 d^4x_3 \, e^{i(q_a x_1 + q_b x_2 - q_c x_3)} \overline{\mathcal{M}}^{ef}_{abcd}(x_j) \tag{6}$$

$$= -\frac{1}{2F^2}\left(\delta^{af}\overset{\circ}{G}{}^{ebcd}(q_j) + \delta^{bf}\overset{\circ}{G}{}^{aecd}(q_j) + \delta^{cf}\overset{\circ}{G}{}^{abed}(q_j) + \delta^{df}\overset{\circ}{G}{}^{abce}(q_j) + (e \leftrightarrow f) + \ldots\right),$$

where the $\circ$ indicates that the quantity is taken in the chiral limit. Again, the dots stand for terms without the four pion poles.

### B. Quark-mass logarithms

We are interested in the leading logarithm in the quark-mass expansion of $T^{abcd}(s,t)$, i.e. terms of the form $f(s,t)M^2 \log M^2$, where $f(s,t)$ has no quark-mass dependence, and $M^2 = 2Bm_\ell$, where $m_\ell$ is the $\ell$ight quark mass ($m_u = m_d = m_\ell$), and $B$ is a low-energy constant, related to the quark condensate in the chiral limit. First, we note the quark-mass expansions [1]

$$M_\pi^2 = M^2 + \mathcal{O}(M^4 \log M^2)\,, \quad F_\pi = F + \mathcal{O}(M^2 \log M^2)\,, \tag{7}$$
$$G_\pi = 2BF\left(1 - \frac{M^2}{32\pi^2 F^2}\log M^2 + \ldots\right)\,, \tag{8}$$

where the dots in the last equation stands for terms analytic or of higher order in $M^2$. Following the general argument of [3], and based on the examination of Feynman graphs contributing to the four-point function in ChPT, we expect that the leading quark-mass logarithm in $G^{abcd}(q_j)$ is generated in the loop integral (employing dimensional regularization)

$$I^{abcd}_{\log}(q_j) = \frac{1}{2}\int \frac{d^dp}{(2\pi)^d}\frac{i\delta^{ef}\overline{M}{}^{ef}_{abcd}(q_j)}{p^2 - M^2} = -\frac{1}{2F^2}\left(4\overset{\circ}{G}{}^{abcd}(q_j) + \ldots\right)\frac{M^2}{16\pi^2}\log M^2 + \mathcal{O}(M^2) \tag{9}$$

for spacetime dimension $d \to 4$ (summation over $e, f$ is implied in the above expression). Graphically, these corrections correspond to the pion loop graphs of the form of Fig. 1. There are graphs where both ends of the extracted pion line are attached to one of the pion lines connecting one of the $P^j$ operator insertions to the rest of the diagram (they are related to pole graphs $\sim 1/q_j^2$ in the process $\pi^a\pi^b\pi^e \to \pi^c\pi^d\pi^f$ in the chiral limit). We note that these line insertions are of the form

$$\sim \frac{1}{q^2}\left(q^2 \cdot f(q^2)\cdot\left(M^2\log M^2 + \mathcal{O}(M^2)\right)\right)\frac{1}{q^2}\,, \quad f(q^2) \to \text{const.} \quad \text{for} \quad q^2 \to 0\,,$$

for reasons of the usual ChPT power counting, and so these insertions just yield wave-function renormalization corrections of the form $\sim$ const. $(M^2 \log M^2 + \mathcal{O}(M^2))$, which are absorbed in the corrections to $\overset{\circ}{G}_\pi$, $\overset{\circ}{T}{}^{abcd}$, etc. The pole positions are not shifted by those $M^2 \log M^2$ corrections, in accord with Eq. (7). But even if they were shifted, that would not matter in our

argument, since we are only interested in the residues of those poles here.

The second kind of pole graphs for $\pi^a(q_a)\pi^b(q_b)\pi^e(p) \to \pi^c(q_c)\pi^d(q_d)\pi^f(p')$, when $p, p' \to 0$, which can not be dealt with in terms of wave-function renormalization, are the propagator poles $\sim 1/s$, $1/t$, $1/u$, . These will spoil the argument involving the integral in Eq. (9) when they become singular (as $s, t$, or $u \to 0$), since the integrand becomes singular in this case. So, in the case where one of these Mandelstam variables vanishes, the following arguments are not valid, and we exclude these cases from now on. In all other situations, however, the argument should be valid, as there are no additional classes of pole graphs for $p, p' \to 0$.

Extracting now the diagrams with a quadruple pion pole in Eq. (9), we find that the leading logarithmic quark-mass corrections in $G^{abcd}_{\rm res}(q_j)$ modify this part of the four-point function as

$$\begin{aligned} G^{abcd}_{\rm res}(q_j) &= \mathring{G}^{abcd}_{\rm res}(q_j) - \frac{4}{2F^2}\mathring{G}^{abcd}(q_j)\frac{M^2}{16\pi^2}\log M^2 + \mathcal{O}(M^2) \\ &= \mathring{G}^4_\pi \mathring{T}^{abcd}(s,t) - \frac{4}{2F^2}\left(\mathring{G}^4_\pi \mathring{T}^{abcd}(s,t)\right)\frac{M^2}{16\pi^2}\log M^2 + \mathcal{O}(M^2) \\ &= \mathring{G}^4_\pi \mathring{T}^{abcd}(s,t)\left(1 - \frac{4}{2F^2}\frac{M^2}{16\pi^2}\log M^2 + \mathcal{O}(M^2)\right) \\ &\overset{(8)}{=} G^4_\pi\left(\mathring{T}^{abcd}(s,t) + \mathcal{O}(M^2)\right) \overset{!}{=} G^4_\pi T^{abcd}(s,t)\,, \end{aligned} \tag{10}$$

compare Eq. (2). So we see that no corrections of the form $\sim M^2\log M^2$ are left for the scattering amplitude. The quark-mass logarithms in the scattering amplitude must therefore be accompanied by powers $M^4$ or higher (except for the cases where one of $s, t, u$ vanishes, or is fixed at a value of $\mathcal{O}(M^2)$).

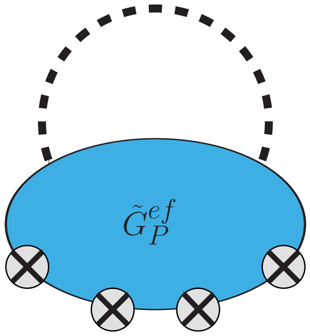


FIG. 1: Symbolical representation of the class of Feynman graphs which generates the leading quark-mass logarithm of the pseudoscalar four-point function. The crossed circles denote $P$ operator insertions, the dashed line represents a pseudo-Goldstone boson (pion).

In our demonstration, we made heavy use of the fact that the leading infrared singularities, for generic $s, t, u$, are generated by the graphs with the general topology of Fig. 1, i.e. graphs where the propagator of a single pion line becomes singular in a loop integration. One could also consider infrared singularities which are due to *several* soft pion lines, which would all have to be extracted from the "blob" in the figure. For example, let us consider two soft pion loop lines attached to the blob, with loop momenta $l_1$ and $l_2$. There are now two possibilities: Either $l_1$ and $l_2$ are dependent of another, in the sense that, if $l_1$ is "soft" ($\sim M$), then $l_2$ necessarily becomes soft when a combination of $l_1$ and the "external" momenta $q_j$ assumes a particular value, or they are completely independent of another, i.e. they can be independently integrated over for any value of the $q_j$. In the latter case, one can iterate the argument given above, together with the algebraic procedure explained in the appendix, to find a finite result for the matrix element of four $P$ operators and *four* (instead of just two) external soft pions, yielding simply a result of order $(M^{d-2})^2$ for the leading infrared singularity of the graphs in question, which (for $d \to 4$) is obviously of a different form than the terms we are looking for, and suppressed in the quark-mass counting. The first case, in turn, corresponds to the known threshold singularities for the production of two (or more, in the general case) soft pions, for specific values of invariant combinations of the $q_j$. This is clear from the well-known analysis of singularities of Feynman graphs as first given by Landau and Cutkosky. Such specific values of invariant combinations constructed from the $q_j$ are considered as "non-generic" here, and have been excluded in our "caveat" explained on the previous page.

## APPENDIX A: DERIVATION OF SOFT-PION THEOREMS

In this appendix, we employ the method of soft-pion theorems (see [4–8], or e.g. [9] and Sec. 11.3 of [10] for textbook treatments), to demonstrate some general relations between limiting values of matrix elements studied in this work. To this end, we neglect the pion mass and treat only the chiral limit, so that the isovector axial-vector current is also conserved (in addition to the vector current). We assume that the matrix elements considered here do not diverge in the chiral limit. First, we note that the quark currents $V, A, S, P$ (defined as in [1, 2]) obey the algebra

$$
\begin{aligned}
[A_0^i(z), A_\rho^j(z')]_{z^0=z'^0} &= i\epsilon^{ijk} V_\rho^k(z)\delta^3(\vec{z}-\vec{z}')\,, & [A_0^i(z), V_\rho^j(z')]_{z^0=z'^0} &= i\epsilon^{ijk} A_\rho^k(z)\delta^3(\vec{z}-\vec{z}')\,,\\
[V_0^i(z), A_\rho^j(z')]_{z^0=z'^0} &= i\epsilon^{ijk} A_\rho^k(z)\delta^3(\vec{z}-\vec{z}')\,, & [V_0^i(z), V_\rho^j(z')]_{z^0=z'^0} &= i\epsilon^{ijk} V_\rho^k(z)\delta^3(\vec{z}-\vec{z}')\,,\\
[A_0^i(z), S^j(z')]_{z^0=z'^0} &= i\delta^{ij} P^0(z)\delta^3(\vec{z}-\vec{z}')\,, & [A_0^i(z), P^j(z')]_{z^0=z'^0} &= -i\delta^{ij} S^0(z)\delta^3(\vec{z}-\vec{z}')\,,\\
[A_0^i(z), S^0(z')]_{z^0=z'^0} &= iP^i(z)\delta^3(\vec{z}-\vec{z}')\,, & [A_0^i(z), P^0(z')]_{z^0=z'^0} &= -iS^i(z)\delta^3(\vec{z}-\vec{z}')\,,
\end{aligned}
$$

where summation over the isospin index $k = 1, 2, 3$ is implied, and $S^0$, $P^0$ denote the isoscalar currents. See e.g. [2], Sec. 2.4, for the explicit calculation of such commutators.

We want to find a formula for pion matrix elements of time-ordered products of local operators $O_n(x_n)$,

$$\langle \pi^j(p')|TO_1(x_1)O_2(x_2)\dots O_n(x_n)|\pi^i(p)\rangle\,,$$

in the limit where the pion four-momenta approach zero. The above matrix elements corresponds to the sum of all Feynman graphs with an incoming pion $\pi^i(p)$, an outgoing pion $\pi^j(p')$, and $n$ operator insertions at fixed space-time positions $x_m$ (see e.g. Sec. 6.4 of [11]). It is thus clear from crossing symmetry that this matrix element will be symmetric under simultaneous exchange of $p \leftrightarrow -p'$, $i \leftrightarrow j$, so that we can always symmetrize in the cartesian isospin indices $i, j$ as we are only interested in the limit $p, p' \to 0$.

We then consider the following Fourier-transformed matrix element:

$$M_{\rho\sigma}^{ji}(x, y, p', p) := \frac{1}{2}\int d^4z' \int d^4z\, e^{ip'z'} e^{-ipz} \langle 0|TA_\rho^j(z')A_\sigma^i(z)O_1(x_1)\dots O_n(x_n)|0\rangle + (i \leftrightarrow j)\,. \tag{A.1}$$

Since the axial-vector operator can generate a single pion,

$$\langle 0|A_\sigma^i(z)|\pi^k(p)\rangle = iF\delta^{ik} p_\sigma e^{-ipz}\,, \tag{A.2}$$

we expect that $M^{ji}_{\rho\sigma}$ has pion poles in $p^2$ and $p'^2$, which can be extracted *à la* LSZ [12] (using translation invariance),

$$M^{ji}_{00}(x,y,p',p)|_{\vec{p}'\to 0,\vec{p}\to 0} = \langle 0|A^j_0(0)|\pi^j\rangle \frac{i}{(p'^0)^2}\langle \pi^j|TO_1(x_1)\dots O_n(x_n)|\pi^i\rangle \frac{i}{(p^0)^2}\langle \pi^i|A^i_0(0)|0\rangle + \dots\,, \tag{A.3}$$

where the dots at the end stand for terms without the double pole, and no summation over $i,j$ is implied in the previous equation. The factor between the pole terms is just the desired matrix element in the limit $M_\pi \to 0$, $p,p' \to 0$. From Eqs. (A.2) and (A.3), we see that $p'^\rho p^\sigma M^{ji}_{\rho\sigma}$ is finite in the limit as $p,p'\to 0$, and just gives the pole terms. So we compute

$$\begin{aligned}
p'^\rho p^\sigma M^{ji}_{\rho\sigma} &= \frac{1}{2}\int d^4z' \int d^4z \left(\partial^\rho_{z'} e^{ip'z'}\right)\left(\partial^\sigma_z e^{-ipz}\right)\langle 0|TA^j_\rho(z')A^i_\sigma(z)O_1(x_1)\dots O_n(x_n)|0\rangle + (i\leftrightarrow j)\\
&= \frac{1}{2}\int d^4z' \int d^4z\, e^{ip'z'}e^{-ipz}\partial^\rho_{z'}\partial^\sigma_z\langle 0|TA^j_\rho(z')A^i_\sigma(z)O_1(x_1)\dots O_n(x_n)|0\rangle + (i\leftrightarrow j)\,.
\end{aligned}$$

Taking the derivatives (noting the current conservation $\partial^\sigma_z A^i_\sigma(z) = 0$), one generates a string of matrix elements of commutators with the axial currents. The equal-time commutators stem from the derivatives of the theta functions which are implicit in the time-ordering operation $T$. Symmetrizing in $i,j$ as indicated above, the result is of the form

$$\begin{aligned}
p'^\rho p^\sigma M^{ji}_{\rho\sigma} &= \int d^4z' \int d^4z\, e^{ip'z'}e^{-ipz}\,\times\\
\times\Bigg(&\frac{1}{2}\sum_{m=1}^{n}\langle 0|TO_1(x_1)\dots[A^j_0(z'),[A^i_0(z),O_m(x_m)]]\dots O_n(x_n)|0\rangle\delta(z'^0-x^0_m)\delta(z^0-x^0_m)\\
&+\frac{1}{2}\sum_{m=1}^{n}\langle 0|TO_1(x_1)\dots[A^i_0(z'),[A^j_0(z),O_m(x_m)]]\dots O_n(x_n)|0\rangle\delta(z'^0-x^0_m)\delta(z^0-x^0_m)\\
&+\frac{1}{2}\sum_{\substack{m,m'=1\\ m'\neq m}}^{n}\langle 0|TO_1(x_1)\dots[A^j_0(z'),O_m(x_m)]\dots[A^i_0(z),O_{m'}(x_{m'})]\dots O_n(x_n)|0\rangle\delta(z'^0-x^0_m)\delta(z^0-x^0_{m'})\\
&+\frac{1}{2}\sum_{\substack{m,m'=1\\ m'\neq m}}^{n}\langle 0|TO_1(x_1)\dots[A^i_0(z'),O_m(x_m)]\dots[A^j_0(z),O_{m'}(x_{m'})]\dots O_n(x_n)|0\rangle\delta(z'^0-x^0_m)\delta(z^0-x^0_{m'})\Bigg)\,.
\end{aligned}$$

Taking the limit $\vec{p}'\to 0, \vec{p}\to 0$ in the last equation, and defining the axial charge as

$$Q^i_A(t) := \int d^3\vec{z}\, A^i_0(\vec{z},t)\,, \tag{A.4}$$

we can perform all spacetime integrations, and compare the result for $p'^0 p^0 M^{ji}_{00}$ with Eq. (A.3). The final result is a sum of matrix elements of double or single commutators of the operators $O_m(x_m)$ with the axial charge:

$$
\begin{aligned}
&-F^2\langle\pi^j(p')|TO_1(x_1)\ldots O_n(x_n)|\pi^i(p)\rangle_{M_\pi,p,p'\to 0}\\
&=\frac{1}{2}\sum_{m=1}^{n}\langle 0|TO_1(x_1)\ldots[Q_A^j(x_m^0),[Q_A^i(x_m^0),O_m(x_m)]]\ldots O_n(x_n)|0\rangle\\
&+\frac{1}{2}\sum_{m=1}^{n}\langle 0|TO_1(x_1)\ldots[Q_A^i(x_m^0),[Q_A^j(x_m^0),O_m(x_m)]]\ldots O_n(x_n)|0\rangle\\
&+\sum_{\substack{m,m'=1\\ m'\neq m}}^{n}\langle 0|TO_1(x_1)\ldots[Q_A^j(x_m^0),O_m(x_m)]\ldots[Q_A^i(x_{m'}^0),O_{m'}(x_{m'})]\ldots O_n(x_n)|0\rangle\,.
\end{aligned}
$$

With $[Q_A^i(x^0),P^k(x)]=-i\delta^{ik}S^0(x),$ and $[Q_A^i(x^0),S^0(x)]=iP^i(x)$, we find explicitly:

$$
\begin{aligned}
-F^2\overline{\mathcal{M}}^{ef}_{abcd}(x_j) &= -F^2\mathrm{lim}_{p,p'\to 0}\mathrm{lim}_{M_\pi\to 0}\mathcal{M}^{ef}_{abcd}(x_j) \qquad \text{(A.5)}\\
&=\frac{1}{2}\Big(\delta^{af}\langle 0|TP^e(x_1)P^b(x_2)P^c(x_3)P^d(0)|0\rangle+\delta^{bf}\langle 0|TP^a(x_1)P^e(x_2)P^c(x_3)P^d(0)|0\rangle\\
&+\delta^{cf}\langle 0|TP^a(x_1)P^b(x_2)P^e(x_3)P^d(0)|0\rangle+\delta^{df}\langle 0|TP^a(x_1)P^b(x_2)P^c(x_3)P^e(0)|0\rangle\\
&+\delta^{ae}\langle 0|TP^f(x_1)P^b(x_2)P^c(x_3)P^d(0)|0\rangle+\delta^{be}\langle 0|TP^a(x_1)P^f(x_2)P^c(x_3)P^d(0)|0\rangle\\
&+\delta^{ce}\langle 0|TP^a(x_1)P^b(x_2)P^f(x_3)P^d(0)|0\rangle+\delta^{de}\langle 0|TP^a(x_1)P^b(x_2)P^c(x_3)P^f(0)|0\rangle\Big)\\
&-\Big((\delta^{ae}\delta^{bf}+\delta^{af}\delta^{be})\langle 0|TS^0(x_1)S^0(x_2)P^c(x_3)P^d(0)|0\rangle\\
&\quad+(\delta^{ae}\delta^{cf}+\delta^{af}\delta^{ce})\langle 0|TS^0(x_1)P^b(x_2)S^0(x_3)P^d(0)|0\rangle\\
&\quad+(\delta^{ae}\delta^{df}+\delta^{af}\delta^{de})\langle 0|TS^0(x_1)P^b(x_2)P^c(x_3)S^0(0)|0\rangle\\
&\quad+(\delta^{be}\delta^{cf}+\delta^{bf}\delta^{ce})\langle 0|TP^a(x_1)S^0(x_2)S^0(x_3)P^d(0)|0\rangle\\
&\quad+(\delta^{be}\delta^{df}+\delta^{bf}\delta^{de})\langle 0|TP^a(x_1)S^0(x_2)P^c(x_3)S^0(0)|0\rangle\\
&\quad+(\delta^{ce}\delta^{df}+\delta^{cf}\delta^{de})\langle 0|TP^a(x_1)P^b(x_2)S^0(x_3)S^0(0)|0\rangle\Big)\,,
\end{aligned}
$$

for the matrix element of Eq. (4), with all correlators taken in the chiral limit. The correlators involving two $S^0$ operators do not lead to four pion poles (one for each $q_j^2$ in the Fourier transform), since the $S^0$ operator cannot generate a single pion. So the only relevant terms for us here are the correlators involving four pseudoscalar currents.

## APPENDIX B: TREE GRAPHS WITH POLES FOR $\overline{\mathcal{M}}^{\mathbf{ef}}_{\mathbf{abcd}}(\mathbf{x_j})$

We evaluate the tree graphs from $\mathcal{L}^{(2)}_{\text{ChPT}}$ with four pion poles, in the exponential parameterization, $U = \exp(i\pi^a\tau^a/F)$, which contribute to $\langle\pi^f(p')|TP^a(x_1)P^b(x_2)P^c(x_3)P^d(0)|\pi^e(p)\rangle$ in the chiral limit, for $p, p' \to 0$. We give the momentum-space Feynman rules, neglecting terms which do not contribute to the residues at the poles in $q_j^2$.

Two graphs with a pole in the $s$-channel:

$$G_s = (2iBF)^4 \left(\prod_{j=a}^{d} \frac{i}{q_j^2}\right)\left(-\frac{is}{9F^4}\right)\Big(8\delta^{ab}\delta^{cd}\delta^{ef} - 4\delta^{ab}\left(\delta^{cf}\delta^{de} + \delta^{ce}\delta^{df}\right) - 4\delta^{cd}\left(\delta^{ae}\delta^{bf} + \delta^{af}\delta^{be}\right)$$
$$+ \delta^{ac}\left(\delta^{be}\delta^{df} + \delta^{bf}\delta^{de}\right) + \delta^{ad}\left(\delta^{be}\delta^{cf} + \delta^{bf}\delta^{ce}\right) + \delta^{ae}\left(\delta^{bc}\delta^{df} + \delta^{bd}\delta^{cf}\right) + \delta^{af}\left(\delta^{bc}\delta^{de} + \delta^{bd}\delta^{ce}\right)\Big) .$$

Two graphs with a pole in the $t$-channel:

$$G_t = (2iBF)^4 \left(\prod_{j=a}^{d} \frac{i}{q_j^2}\right)\left(-\frac{it}{9F^4}\right)\Big(8\delta^{ac}\delta^{bd}\delta^{ef} - 4\delta^{ac}\left(\delta^{bf}\delta^{de} + \delta^{be}\delta^{df}\right) - 4\delta^{bd}\left(\delta^{ae}\delta^{cf} + \delta^{af}\delta^{ce}\right)$$
$$+ \delta^{ab}\left(\delta^{ce}\delta^{df} + \delta^{cf}\delta^{de}\right) + \delta^{ad}\left(\delta^{ce}\delta^{bf} + \delta^{cf}\delta^{be}\right) + \delta^{ae}\left(\delta^{bc}\delta^{df} + \delta^{cd}\delta^{bf}\right) + \delta^{af}\left(\delta^{bc}\delta^{de} + \delta^{cd}\delta^{be}\right)\Big) .$$

Two graphs with a pole in the $u$-channel:

$$G_u = (2iBF)^4 \left(\prod_{j=a}^{d} \frac{i}{q_j^2}\right)\left(-\frac{iu}{9F^4}\right)\Big(8\delta^{ad}\delta^{bc}\delta^{ef} - 4\delta^{ad}\left(\delta^{cf}\delta^{be} + \delta^{ce}\delta^{bf}\right) - 4\delta^{bc}\left(\delta^{ae}\delta^{df} + \delta^{af}\delta^{de}\right)$$
$$+ \delta^{ab}\left(\delta^{de}\delta^{cf} + \delta^{df}\delta^{ce}\right) + \delta^{ac}\left(\delta^{de}\delta^{bf} + \delta^{df}\delta^{be}\right) + \delta^{ae}\left(\delta^{cd}\delta^{bf} + \delta^{bd}\delta^{cf}\right) + \delta^{af}\left(\delta^{cd}\delta^{be} + \delta^{bd}\delta^{ce}\right)\Big) .$$

Note that the poles in $s, t, u$ are not present in the residues.

Four graphs with a pole in $q_j^2$:

$$G_{\text{brems}} = (2iBF)^4 \left(\prod_{j=a}^{d} \frac{i}{q_j^2}\right)\left(\frac{i}{3F^2}\right)\Big(8\delta^{ef}\mathring{T}_2^{abcd} - \delta^{ae}\mathring{T}_2^{fbcd} - \delta^{af}\mathring{T}_2^{ebcd} - \delta^{be}\mathring{T}_2^{afcd} - \delta^{bf}\mathring{T}_2^{aecd}$$
$$- \delta^{ce}\mathring{T}_2^{abfd} - \delta^{cf}\mathring{T}_2^{abed} - \delta^{de}\mathring{T}_2^{abcf} - \delta^{df}\mathring{T}_2^{abce}\Big) ,$$

where

$$\mathring{T}_2^{abcd} = \frac{1}{F^2}\left(\delta^{ab}\delta^{cd}s + \delta^{ac}\delta^{bd}t + \delta^{ad}\delta^{bc}u\right) .$$

There are no double poles in the $q_j^2$, for reasons explained in the main text.

Four graphs with $\pi^e, \pi^f$ coupling to $P(x)$ operators:

$$G_{\rm op} = (2iBF)^4 \left(\prod_{j=a}^{d} \frac{i}{q_j^2}\right) \left(-\frac{i}{3F^2}\right) \Big(4\delta^{ef} \overset{\circ}{T}{}_2^{abcd} + \delta^{ae} \overset{\circ}{T}{}_2^{fbcd} + \delta^{af} \overset{\circ}{T}{}_2^{ebcd} + \delta^{be} \overset{\circ}{T}{}_2^{afcd} + \delta^{bf} \overset{\circ}{T}{}_2^{aecd}$$
$$+ \delta^{ce} \overset{\circ}{T}{}_2^{abfd} + \delta^{cf} \overset{\circ}{T}{}_2^{abed} + \delta^{de} \overset{\circ}{T}{}_2^{abcf} + \delta^{df} \overset{\circ}{T}{}_2^{abce}\Big) \, .$$

Graph with $\pi^6$ vertex:

$$G_{6\pi} = (2iBF)^4 \left(\prod_{j=a}^{d} \frac{i}{q_j^2}\right) \left(-\frac{i}{9F^2}\right) \Big(4\delta^{ef} \overset{\circ}{T}{}_2^{abcd} + \delta^{ae} \overset{\circ}{T}{}_2^{fbcd} + \delta^{af} \overset{\circ}{T}{}_2^{ebcd} + \delta^{be} \overset{\circ}{T}{}_2^{afcd} + \delta^{bf} \overset{\circ}{T}{}_2^{aecd}$$
$$+ \delta^{ce} \overset{\circ}{T}{}_2^{abfd} + \delta^{cf} \overset{\circ}{T}{}_2^{abed} + \delta^{de} \overset{\circ}{T}{}_2^{abcf} + \delta^{df} \overset{\circ}{T}{}_2^{abce}\Big) \, .$$

In summa:

First, the graphs with the $s, t, u$-channel one-pion exchanges can be combined to give

$$G_s + G_t + G_u = (2iBF)^4 \left(\prod_{j=a}^{d} \frac{i}{q_j^2}\right) \left(-\frac{i}{9F^2}\right) \Big(8\delta^{ef} \overset{\circ}{T}{}_2^{abcd} - \frac{5}{2}\Big(\delta^{ae} \overset{\circ}{T}{}_2^{fbcd} + \delta^{af} \overset{\circ}{T}{}_2^{ebcd} + \delta^{be} \overset{\circ}{T}{}_2^{afcd}$$
$$+ \delta^{bf} \overset{\circ}{T}{}_2^{aecd} + \delta^{ce} \overset{\circ}{T}{}_2^{abfd} + \delta^{cf} \overset{\circ}{T}{}_2^{abed} + \delta^{de} \overset{\circ}{T}{}_2^{abcf} + \delta^{df} \overset{\circ}{T}{}_2^{abce}\Big)\Big) \, .$$

The terms $\sim \delta^{ef}$ cancel in the sum of all graphs. The remainder yields

$$G_s + G_t + G_u + G_{\rm brems} + G_{\rm op} + G_{6\pi} \tag{B.1}$$
$$= -\frac{1}{2F^2}\Big[i(2iBF)^4 \left(\prod_{j=a}^{d} \frac{i}{q_j^2}\right) \Big(\delta^{ae} \overset{\circ}{T}{}_2^{fbcd} + \delta^{af} \overset{\circ}{T}{}_2^{ebcd} + \delta^{be} \overset{\circ}{T}{}_2^{afcd} + \delta^{bf} \overset{\circ}{T}{}_2^{aecd} + \delta^{ce} \overset{\circ}{T}{}_2^{abfd}$$
$$+ \delta^{cf} \overset{\circ}{T}{}_2^{abed} + \delta^{de} \overset{\circ}{T}{}_2^{abcf} + \delta^{df} \overset{\circ}{T}{}_2^{abce}\Big)\Big] \, .$$

This corresponds exactly to the pole terms of Eq. (A.5), which is what we wanted to show here.

[1] J. Gasser and H. Leutwyler, Annals Phys. **158** (1984) 142.

[2] S. Scherer, Adv. Nucl. Phys. **27** (2003) 277 [hep-ph/0210398].

[3] L. F. Li and H. Pagels, Phys. Rev. Lett. **26**, 1204 (1971).

[4] Y. Nambu and D. Lurie, Phys. Rev. **125** (1962) 1429.

[5] S. L. Adler, Phys. Rev. **137** (1965) B1022.

[6] S. L. Adler, Phys. Rev. **139** (1965) B1638.

[7] S. Weinberg, Phys. Rev. Lett. **18** (1967) 188.

[8] R. F. Dashen and M. Weinstein, Phys. Rev. **183** (1969) 1261.

[9] D. H. Lyth, "An Introduction to Current Algebra", Oxford, UK: Clarendon Press (1970).

[10] C. Itzykson and J. B. Zuber, "Quantum Field Theory", New York, USA: McGraw-Hill (1980).

[11] S. Weinberg, "The Quantum Theory of Fields. Vol. 1: Foundations", Cambridge, UK: Univ. Pr. (1995).

[12] H. Lehmann, K. Symanzik and W. Zimmermann, Nuovo Cim. **1** (1955) 205.
